# Supplementary material for: Learning Inference Models for Computer Vision
Source: arXiv:1709.00069 source file (2017-08-31)
Supplement: Supplementary file 2 [file appendix4.tex]

\chapter{Additional Results for Consensus Message Passing}

\section{Additional results on the face problem}

\subsection{Qualitative results}

Figure~\ref{fig:shading-qualitative-multiple-subjects} shows inference results for reflectance maps, normal maps and lights for randomly chosen test images, and Figure~\ref{fig:shading-qualitative-same-subject} shows reflectance estimation results on multiple images of the same subject produced under different illumination conditions. \Method is able to produce reflectance estimates that are closer to the photometric stereo groundtruth across subjects and across different illumination conditions.

\subsection{Quantitative results}

Figure~\ref{fig:shading-quantitative-reflectance} shows quantitative results for both real images from `Yale B' and `Extended Yale B' datasets \citep{Georghiades2001, Lee2005} and synthetic shadowless images. The synthetic shadowless images were created using the same light, reflectance and normal map statistics as that of images in the real dataset (however estimated using photometric stereo~\citep{Queau2013}). Subject recognition results indicate superior performance of \MTD in comparison to other baselines in both real and synthetic image settings.

Figure~\ref{fig:shading-quantitative-light} shows the quantitative results of light inference using the different inference techniques. We use the cosine angle distance between the estimated light and the photometric stereo groundtruth ($\textrm{error} = \cos^{-1}(\hat{\mathbf{l}}_\textrm{est}.\hat{\mathbf{l}}_\textrm{ps})$) as an error metric. Here, $\hat{\mathbf{l}}_\textrm{est}$ is a unit vector in the same direction as the mean of the posterior light estimate of \MTD and $\hat{\mathbf{l}}_\textrm{ps}$ is a unit vector in the same direction as the corresponding photometric stereo groundtruth. Again, these results indicate the superior performance of \MTD in comparison to other baselines in both real and synthetic image settings.

\begin{figure*}[h]
	\centering
	\setlength\fboxsep{0.2mm}
	\setlength\fboxrule{0pt}
	\begin{tikzpicture}

	\node at (-7.3, 2.9) {\small (a) Observed};
	\node at (-4.2, 2.9) {\small (b) Reflectance};
	\node at (-0.58, 2.9) {\small (c) Variance};
	\node at (2.35, 2.9) {\small (d) Light};
	\node at (6.4, 2.9) {\small (e) Normal};

	\node at (-4.15, 2.6) {\tiny $\color{gray}{\overbrace{\quad\quad\quad\quad\quad\quad\quad\quad\quad\quad
														  \quad\quad\quad\quad\quad\quad\quad\quad\quad\quad
														  \quad\quad\quad\quad\quad\quad}}$};

    \node at (2.45, 2.6) {\tiny $\color{gray}{\overbrace{\quad\quad\quad\quad\quad\quad\quad\quad\quad\quad
														 \quad\quad\quad\quad\quad\quad\quad\quad\quad\quad}}$};

	\node at (6.58, 2.6) {\tiny $\color{gray}{\overbrace{\quad\quad\quad\quad\quad\quad\quad\quad\quad\quad
														 \quad\quad\quad\quad\quad\,\,\,}}$};

		\matrix at (0, 0) [matrix of nodes, nodes={anchor=east}, column sep=-0.15cm, row sep=-0.2cm]
		{
			\fbox{\includegraphics[width=1cm]{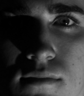}} & \hspace{0.12cm} &
			\fbox{\includegraphics[width=1cm]{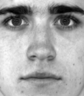}} &
			\fbox{\includegraphics[width=1cm]{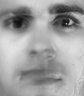}} &
			\fbox{\includegraphics[width=1cm]{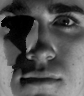}} &
			\fbox{\includegraphics[width=1cm]{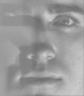}}  &
			\fbox{\includegraphics[width=1cm]{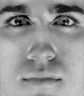}} & \hspace{0.12cm} &
			\fbox{\includegraphics[width=1cm]{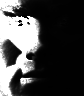}} & \hspace{0.12cm} &
			\fbox{\includegraphics[width=1cm]{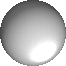}} &
			\fbox{\includegraphics[width=1cm]{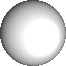}} &
			\fbox{\includegraphics[width=1cm]{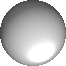}}  &
			\fbox{\includegraphics[width=1cm]{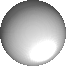}} & \hspace{0.12cm} &
			\fbox{\includegraphics[width=1cm]{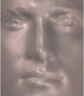}} &
			\fbox{\includegraphics[width=1cm]{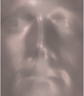}} &
			\fbox{\includegraphics[width=1cm]{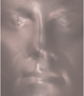}}  	\\

			\fbox{\includegraphics[width=1cm]{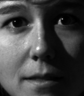}} & \hspace{0.12cm} &
			\fbox{\includegraphics[width=1cm]{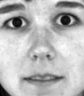}} &
			\fbox{\includegraphics[width=1cm]{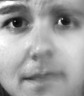}} &
			\fbox{\includegraphics[width=1cm]{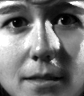}} &
			\fbox{\includegraphics[width=1cm]{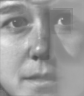}} &
			\fbox{\includegraphics[width=1cm]{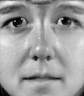}} & \hspace{0.12cm} &
			\fbox{\includegraphics[width=1cm]{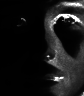}} & \hspace{0.12cm} &
			\fbox{\includegraphics[width=1cm]{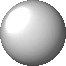}} &
			\fbox{\includegraphics[width=1cm]{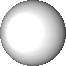}}  &
			\fbox{\includegraphics[width=1cm]{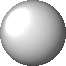}} &
			\fbox{\includegraphics[width=1cm]{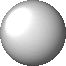}} & \hspace{0.12cm} &
			\fbox{\includegraphics[width=1cm]{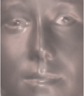}} &
			\fbox{\includegraphics[width=1cm]{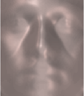}} &
			\fbox{\includegraphics[width=1cm]{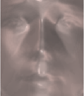}}  \\

			\fbox{\includegraphics[width=1cm]{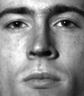}} & \hspace{0.12cm} &
			\fbox{\includegraphics[width=1cm]{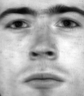}} &
			\fbox{\includegraphics[width=1cm]{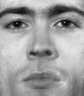}} &
			\fbox{\includegraphics[width=1cm]{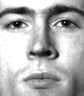}} &
			\fbox{\includegraphics[width=1cm]{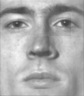}} &
			\fbox{\includegraphics[width=1cm]{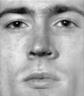}} & \hspace{0.12cm} &
			\fbox{\includegraphics[width=1cm]{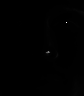}} & \hspace{0.12cm} &
			\fbox{\includegraphics[width=1cm]{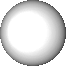}} &
			\fbox{\includegraphics[width=1cm]{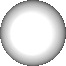}} &
			\fbox{\includegraphics[width=1cm]{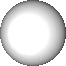}}  &
			\fbox{\includegraphics[width=1cm]{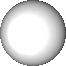}} & \hspace{0.12cm} &
			\fbox{\includegraphics[width=1cm]{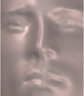}} &
			\fbox{\includegraphics[width=1cm]{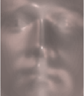}} &
			\fbox{\includegraphics[width=1cm]{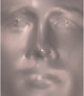}} \\

			\fbox{\includegraphics[width=1cm]{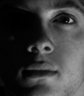}} & \hspace{0.12cm} &
			\fbox{\includegraphics[width=1cm]{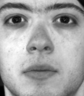}} &
			\fbox{\includegraphics[width=1cm]{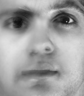}} &
			\fbox{\includegraphics[width=1cm]{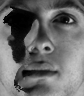}} &
			\fbox{\includegraphics[width=1cm]{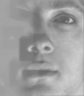}} &
			\fbox{\includegraphics[width=1cm]{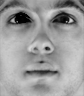}} & \hspace{0.12cm} &
			\fbox{\includegraphics[width=1cm]{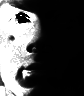}} & \hspace{0.12cm} &
			\fbox{\includegraphics[width=1cm]{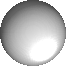}} &
			\fbox{\includegraphics[width=1cm]{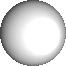}} &
			\fbox{\includegraphics[width=1cm]{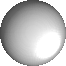}} &
			\fbox{\includegraphics[width=1cm]{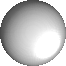}} & \hspace{0.12cm} &
			\fbox{\includegraphics[width=1cm]{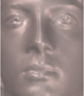}} &
			\fbox{\includegraphics[width=1cm]{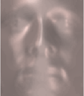}} &
			\fbox{\includegraphics[width=1cm]{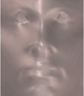}}  \\
	     };

	     \node at (-6.4, -2.7) {\small GT};
	     \node at (-5.25, -2.7) {\small BU};
	     \node at (-4.1, -2.7) {\small MP};
	     \node at (-3.0, -2.7) {\small Forest};
	     \node at (-1.87, -2.7) {\small \textbf{CMP}};

	     \node at (-0.55, -2.7) {\small \textbf{CMP}};

	     \node at (0.75, -2.7) {\small GT};
	     \node at (1.9, -2.7) {\small MP};
	     \node at (3, -2.7) {\small Forest};
	     \node at (4.15, -2.7) {\small \textbf{CMP}};

	     \node at (5.5, -2.7) {\small GT};
	     \node at (6.6, -2.7) {\small MP};
	     \node at (7.72, -2.7) {\small \textbf{CMP}};

	\end{tikzpicture}
	\vspace{-0.4cm}
	\mycaption{A visual comparison of inference results}{For 4 randomly chosen test images, we show inference results obtained by competing methods. (a)~Observed images. (b)~Inferred reflectance maps. \textit{GT} is the photometric stereo groundtruth, \textit{BU} is the Biswas \etal (2009) reflectance estimate and \textit{Forest} is the consensus prediction. (c)~The variance of the inferred reflectance estimate produced by \MTD (normalized across rows). High variance regions correlate strongly with cast shadows. (d)~Visualization of inferred light directions. (e)~Inferred normal maps.}
	\label{fig:shading-qualitative-multiple-subjects-supp}
\end{figure*}

\begin{figure*}[H]
	\centering
	\setlength\fboxsep{0.2mm}
	\setlength\fboxrule{0pt}
	\begin{tikzpicture}

		\matrix at (0, 0) [matrix of nodes, nodes={anchor=east}, column sep=-0.15cm, row sep=-0.2cm]
		{
			\fbox{\includegraphics[width=1cm]{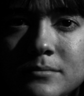}} &
			\fbox{\includegraphics[width=1cm]{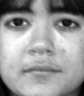}} &
			\fbox{\includegraphics[width=1cm]{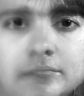}}  &
			\fbox{\includegraphics[width=1cm]{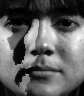}}  &
			\fbox{\includegraphics[width=1cm]{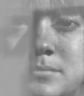}}  &
			\fbox{\includegraphics[width=1cm]{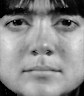}}  &
			\fbox{\includegraphics[width=1cm]{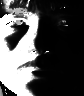}} & \hspace{0.25cm} &

			\fbox{\includegraphics[width=1cm]{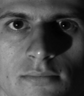}} &
			\fbox{\includegraphics[width=1cm]{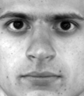}} &
			\fbox{\includegraphics[width=1cm]{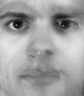}}  &
			\fbox{\includegraphics[width=1cm]{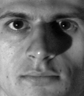}}  &
			\fbox{\includegraphics[width=1cm]{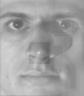}}  &
			\fbox{\includegraphics[width=1cm]{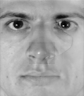}}  &
			\fbox{\includegraphics[width=1cm]{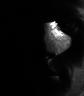}}
			 \\

			\fbox{\includegraphics[width=1cm]{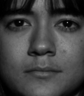}} &
			\fbox{\includegraphics[width=1cm]{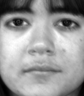}} &
			\fbox{\includegraphics[width=1cm]{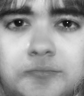}}  &
			\fbox{\includegraphics[width=1cm]{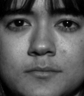}}  &
			\fbox{\includegraphics[width=1cm]{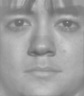}}  &
			\fbox{\includegraphics[width=1cm]{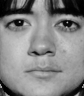}}  &
			\fbox{\includegraphics[width=1cm]{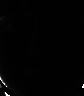}} & \hspace{0.25cm} &

			\fbox{\includegraphics[width=1cm]{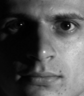}} &
			\fbox{\includegraphics[width=1cm]{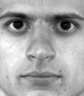}} &
			\fbox{\includegraphics[width=1cm]{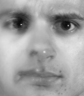}}  &
			\fbox{\includegraphics[width=1cm]{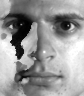}}  &
			\fbox{\includegraphics[width=1cm]{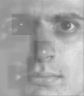}}  &
			\fbox{\includegraphics[width=1cm]{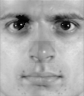}}  &
			\fbox{\includegraphics[width=1cm]{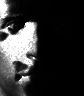}}
			 \\

			\fbox{\includegraphics[width=1cm]{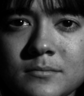}} &
			\fbox{\includegraphics[width=1cm]{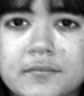}} &
			\fbox{\includegraphics[width=1cm]{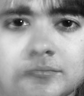}} &
			\fbox{\includegraphics[width=1cm]{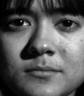}}  &
			\fbox{\includegraphics[width=1cm]{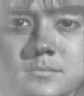}}  &
			\fbox{\includegraphics[width=1cm]{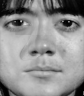}}  &
			\fbox{\includegraphics[width=1cm]{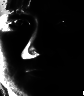}} & \hspace{0.25cm} &

			\fbox{\includegraphics[width=1cm]{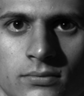}} &
			\fbox{\includegraphics[width=1cm]{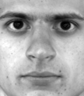}} &
			\fbox{\includegraphics[width=1cm]{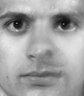}}  &
			\fbox{\includegraphics[width=1cm]{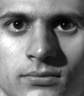}}  &
			\fbox{\includegraphics[width=1cm]{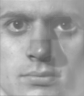}}  &
			\fbox{\includegraphics[width=1cm]{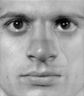}}  &
			\fbox{\includegraphics[width=1cm]{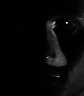}}
			 \\
	     };

	     \node at (-7.47, -2.0) {\small Observed};
	     \node at (-6.33, -2.0) {\small `GT'};
	     \node at (-5.2, -2.0) {\small BU};
	     \node at (-4.1, -2.0) {\small VMP};
	     \node at (-2.95, -2.0) {\small Forest};
	     \node at (-1.87, -2.0) {\small \textbf{CMP}};
	     \node at (-0.75, -2.0) {\small Variance};

	     \node at (0.75, -2.0) {\small Observed};
	     \node at (1.87, -2.0) {\small `GT'};
	     \node at (2.95, -2.0) {\small BU};
	     \node at (4.1, -2.0) {\small VMP};
	     \node at (5.25, -2.0) {\small Forest};
	     \node at (6.35, -2.0) {\small \textbf{CMP}};
	     \node at (7.48, -2.0) {\small Variance};

	\end{tikzpicture}
	\mycaption{Robustness to varying illumination}{Reflectance estimation on two subject images with varying illumination. Left to right: observed image, photometric stereo estimate which is used as a proxy for groundtruth, bottom-up estimate of \cite{Biswas2009}, VMP result, consensus forest estimate, CMP mean, and CMP variance.}
	\label{fig:shading-qualitative-same-subject-supp}
\end{figure*}
